# Supplementary material for: Position: Stop Anthropomorphizing Intermediate Tokens as Reasoning/Thinking Traces!
Source: arXiv:2504.09762 source file (2026-06-09)
Supplement: Supplementary file 1 [file Appendix.tex]

\newpage
\appendix
\section{Appendix}
